# Supplementary material for: Fast non-autoregressive inverse folding with discrete diffusion
Source: arXiv:2312.02447 source file (2023-12-05)
Supplement: Supplementary file 1 [file designability_analysis.tex]

% \begin{table}[]
%     \centering
%     \begin{tabular}{c|c|c}
%         Model & TM-score & RMSD \\
%         \hline
%          PMPNN & 0.9056 & 1.8874 \\
%          \hline
%          Purity Sampling & 0.9036 & 1.9241 \\
%     \end{tabular}
%     \caption{PMPNN versus Diffusion with Purity Sampling Designability For Length-Filtered Test Set \TODO{John, this is good. Can you make this figure over different strides}}
%     \label{tab:filtered_designability}
% \end{table}

% \begin{figure}[h]
%     \centering
%     \includegraphics[scale=0.8]{appendix/tm_score_bins.png}
%     \caption{Average max TM-score binned by sequence length}
%     \label{fig:enter-label}
% \end{figure}
% \begin{figure}[h]
%     \centering
%     \includegraphics[scale=0.8]{appendix/rmsd_bins.png}
%     \caption{Average min RMSD binned by sequence length}
%     \label{fig:enter-label}
% \end{figure}

% \begin{figure}
%     \centering
%     \includegraphics[scale=0.8]{appendix/diversity_vs_rmsd.png}
%     \caption{(WIP) Diversity versus RMSD for PMPNN at different temperatures and Diffusion with different purity prior weights.}
%     \label{fig:enter-label}
% \end{figure}
